# Supplementary material for: Understanding Reduced-Voltage Operation in Modern DRAM Chips: Characterization, Analysis, and Mechanisms
Source: arXiv:1705.10292 source file (2017-05-29)
Supplement: Supplementary file 1 [file appendix_addeq.tex]

% !TEX root=../paper.tex

\appendix
\label{sec:appendix}

\section{FPGA Schematic of DRAM Power Pins}
\label{sec:pin_layout}

\figref{pin_layout} shows all the DRAM power pins connected to the FPGA power
rail that we adjust (see \secref{fpga}). In particular, we tune the VCC1V5 pin,
which is directly connected to all of the $V_{DD}$ and $V_{DDQ}$ pins on the
DIMM. Power pin numbering information can be found on the datasheets provided by
all major vendors (e.g., \cite{micronDDR3L_2Gb, hynix-ddr3l}). The reference
voltage VTTVREF is automatically adjusted by the DRAM to half of VCC1V5.

\figputHW{pin_layout}{DRAM power pins that we adjust.}

\section{Effect of Data Pattern on Error Rate}
\label{sec:datapatt}

As discussed in \ssecref{volt_sensitivity}, we do not observe a significant effect
on the error rate for different data patterns when the supply voltage is reduced.
%\figref{datapatt} shows the average bit error rate (BER) of different data
%patterns across the supply voltage (\vdd) for each vendor. Each data pattern represents the byte
%value (shown in hex) that we fill into the DRAM. For each shown data pattern, we
%also test its bit inversion in the same experiment, as discussed in
%\ssecref{dramtest}.
To compare the impact due to different data patterns,
we conduct a one-way ANOVA to calculate the \emph{p-value} across all
pattern pairs at each voltage step. \tabref{pval} shows the calculated p-value
at each supply voltage step. Supply voltage levels do not have p-values listed in
the table when there are no
errors, or when no reliable latency values can be found.

%\figputWL{datapatt/alt_patt_temp20_trcd4_trp4}{Effect of data patterns on BERs
%  across different supply voltages (\vdd).}{datapatt}

\input{sections/tables/data_patt_pvalue}

The main observation is that using different data patterns does not have a
statistically significant (p-value < 0.05) effect on the error rate at all
supply voltages. Significant effects occur at 1.100V for Vendor~A, at 1.025V for
Vendor~B, and at both 1.250V and 1.100V for Vendor~C. Taken together, these
results suggest that data patterns do not consistently have an effect on errors
induced when the supply voltage is reduced.

\section{DRAM Cell Operation}
\label{dram_cell_op}

In this section, we explain the how the DRAM cell and its state change during
the three fundamental operations: activation, restoration, and precharge
(see \ssecref{access_data}).
\figref{dram_curve} shows the bitline voltage level during these operations with
\vdd set to 1.35V. An \act command and a \pre command are issued at 0ns and 50ns,
respectively. To further help understand the operations, we use
\figref{dram_state} to describe the state of the cell, bitline, and sense
amplifier during the same time frame as \figref{dram_curve}. A bitline is used
to connect a cell with its sense amplifier (in the row buffer) for data
accesses. Accessing data in a DRAM cell consists of four major steps:

\begin{figure}[!h]
    \centering
   \subcaptionbox{DRAM bitline voltage.\label{fig:dram_curve}}
    {
        \includegraphics[width=\columnwidth]{plots/dram_curve}
    }
    \subcaptionbox{DRAM state.\label{fig:dram_state}}
    {
        \includegraphics[width=\columnwidth]{plots/dram_state}
    }
    \caption{DRAM phases during a DRAM access.}
\end{figure}

\paratitle{Precharge} Initially, each cell in the DRAM is in a charged
state (for data value 1) or a discharged state (for data value 0) at 0ns ($T0$). The
amount of filled gray color represents the amount of charge in the cell. In our
shown example, we assume the cell is fully charged, storing a data value of 1.
The bitline voltage is maintained at a voltage of $\frac{1}{2}$\vdd.

\paratitle{Charge Sharing} An \act command connects a row of cells to their
bitlines. This triggers the charge stored in the cells to start flowing to the
bitlines (or the other way around, depending on the initial charge level in the
cell) via a process called \emph{charge sharing} (at time $T1$). In our example,
the cell is initially charged. Hence, it perturbs the bitline's voltage from
$\frac{1}{2}$\vdd to $\frac{1}{2}$\vdd$+\delta$ by a small amount of charge
($\delta$).

\paratitle{Sensing and Amplification} After the charge sharing phase, the
sense amplifier senses the voltage perturbation on the bitline towards either
\vdd or 0. Following the same direction, it starts to amplify the bitline
voltage by injecting more charge into the bitline and the cell. When
the bitline voltage surpasses 75\% of \vdd (at time $T2$), the binary data becomes latched in
the sense amplifier, thus ensuring that the correct data can be read by a \crd
command. These two phases are also known as the activation phase. The activation
latency is the time elapsed from $T0$ to $T2$, which is defined as \trcd.

\paratitle{Restoration} After the row is activated and each sense
amplifier latches in the binary data of its cell, the DRAM starts to restore the
connected cell's charge back to its original fully-charged state (at time $T3$).
This phase is known as restoration, and its latency (from $T0$ to $T3$) is
defined as \tras.

To activate a different row of cells within the same array of the activated row,
the memory controller sends a \pre command to disconnect the cells from the
bitline. Then, the sense amplifier brings the bitline back to $\frac{1}{2}$\vdd
(at time $T4$). The precharge latency is defined at \trp, from the issue time of
\pre (50ns) to $T4$.

\section{Spatial Distribution of Errors}
\label{spatial}

In this section, we expand upon the spatial locality data presented in \ssecref{spatial}.
\figref{full_loc_A}, \figref{full_loc_B}, and \figref{full_loc_C} show the
physical locations of errors that occur when the supply voltage is reduced. At higher voltage levels, even
if errors occur, they tend to cluster in certain regions of a DIMM.
However, as we reduce the supply voltage further, the number of errors increases, and the errors start to
spread across the DIMM.

\begin{figure}[!h]
    \centering
    \subcaptionbox{1.075V.}[0.8\linewidth][l]
    {
        \includegraphics[width=0.8\linewidth]{plots/figs/add_eq/{crucialb41_rcd4_rp4_ret0_temp20_volt1.075000_fix_row_addeq}.pdf}
    }

    \subcaptionbox{1.1V.}[0.8\linewidth][l]
    {
        \includegraphics[width=0.8\linewidth]{plots/figs/add_eq/{crucialb41_rcd4_rp4_ret0_temp20_volt1.100000_fix_row_addeq}.pdf}
    }

    %\subcaptionbox{1.15V.}[0.8\linewidth][l]
    %{
    %    %\includegraphics[width=0.8\linewidth]{plots/figs/add_eq/{crucialb41_rcd4_rp4_ret0_temp20_volt1.150000_fix_row_addeq}.pdf}
    %    \includegraphics[scale=0.5]{plots/figs/{crucialb41_rcd4_rp4_ret0_temp20_volt1.150000_fix_row}.pdf}
    %}
    \caption{Probability of observing errors due to low voltage in a DIMM from Vendor~A.}
    \label{fig:full_loc_A}
\end{figure}
%\figputHS{recompressed}{1}{1}

\begin{figure}[!h]
    \centering
    \subcaptionbox{1.025V.}[0.8\linewidth][l]
    {
        \includegraphics[width=0.8\linewidth]{plots/figs/add_eq/{samsungo13_rcd4_rp4_ret0_temp20_volt1.025000_fix_row_addeq}.pdf}
    }

    \subcaptionbox{1.05V.}[0.8\linewidth][l]
    {
        \includegraphics[width=0.8\linewidth]{plots/figs/add_eq/{samsungo13_rcd4_rp4_ret0_temp20_volt1.050000_fix_row_addeq}.pdf}
    }

    \subcaptionbox{1.1V.}[0.8\linewidth][l]
    {
        \includegraphics[width=0.8\linewidth]{plots/figs/add_eq/{samsungo13_rcd4_rp4_ret0_temp20_volt1.100000_fix_row_addeq}.pdf}
    }
    \caption{Probability of observing errors due to low voltage in a DIMM from Vendor~B.}
    \label{fig:full_loc_B}
\end{figure}

\begin{figure}[!h]
    \centering
    \subcaptionbox{1.1V.}[0.8\linewidth][l]
    {
        \includegraphics[width=0.8\linewidth]{plots/figs/add_eq/{hynixp65_rcd4_rp4_ret0_temp20_volt1.100000_fix_row_addeq}.pdf}
    }
    \subcaptionbox{1.125V.}[0.8\linewidth][l]
    {
        \includegraphics[width=0.8\linewidth]{plots/figs/add_eq/{hynixp65_rcd4_rp4_ret0_temp20_volt1.125000_fix_row_addeq}.pdf}
    }
    \subcaptionbox{1.15V.}[0.8\linewidth][l]
    {
        \includegraphics[width=0.8\linewidth]{plots/figs/add_eq/{hynixp65_rcd4_rp4_ret0_temp20_volt1.150000_fix_row_addeq}.pdf}
    }
    \subcaptionbox{1.175V.}[0.8\linewidth][l]
    {
        \includegraphics[width=0.8\linewidth]{plots/figs/add_eq/{hynixp65_rcd4_rp4_ret0_temp20_volt1.175000_fix_row_addeq}.pdf}
    }
    \subcaptionbox{1.2V.}[0.8\linewidth][l]
    {
        \includegraphics[width=0.8\linewidth]{plots/figs/add_eq/{hynixp65_rcd4_rp4_ret0_temp20_volt1.200000_fix_row_addeq}.pdf}
    }
    \caption{Probability of observing errors due to low voltage in a DIMM from Vendor~C.}
    \label{fig:full_loc_C}
\end{figure}

\ignore{
\begin{figure*}[!h]
    \centering
    \subcaptionbox{1.075V.}[0.31\linewidth][l]
    {
        \includegraphics[width=0.31\linewidth]{plots/figs/{crucialb41_rcd4_rp4_ret0_temp20_volt1.075000_fix_row}.pdf}
    }
    \subcaptionbox{1.1V.}[0.31\linewidth][l]
    {
        \includegraphics[width=0.31\linewidth]{plots/figs/{crucialb41_rcd4_rp4_ret0_temp20_volt1.100000_fix_row}.pdf}
    }
    \subcaptionbox{1.15V.}[0.31\linewidth][l]
    {
        \includegraphics[width=0.31\linewidth]{plots/figs/{crucialb41_rcd4_rp4_ret0_temp20_volt1.150000_fix_row}.pdf}
    }
    \caption{Probability of observing errors due to low voltage in a DIMM from Vendor~A.}
    \label{fig:full_loc_A}
\end{figure*}

\begin{figure*}[!h]
    \centering
    \subcaptionbox{1.025V.}[0.31\linewidth][l]
    {
        \includegraphics[width=0.31\linewidth]{plots/figs/{samsungo13_rcd4_rp4_ret0_temp20_volt1.025000_fix_row}.pdf}
    }
    \subcaptionbox{1.05V.}[0.31\linewidth][l]
    {
        \includegraphics[width=0.31\linewidth]{plots/figs/{samsungo13_rcd4_rp4_ret0_temp20_volt1.050000_fix_row}.pdf}
    }
    \subcaptionbox{1.1V.}[0.31\linewidth][l]
    {
        \includegraphics[width=0.31\linewidth]{plots/figs/{samsungo13_rcd4_rp4_ret0_temp20_volt1.100000_fix_row}.pdf}
    }
    \caption{Probability of observing errors due to low voltage in a DIMM from Vendor~B.}
    \label{fig:full_loc_B}
\end{figure*}

\begin{figure*}[!h]
    \centering
    \subcaptionbox{1.1V.}[0.31\linewidth][l]
    {
        \includegraphics[width=0.31\linewidth]{plots/figs/{hynixp65_rcd4_rp4_ret0_temp20_volt1.100000_fix_row}.pdf}
    }
    \subcaptionbox{1.125V.}[0.31\linewidth][l]
    {
        \includegraphics[width=0.31\linewidth]{plots/figs/{hynixp65_rcd4_rp4_ret0_temp20_volt1.125000_fix_row}.pdf}
    }
    \subcaptionbox{1.15V.}[0.31\linewidth][l]
    {
        \includegraphics[width=0.31\linewidth]{plots/figs/{hynixp65_rcd4_rp4_ret0_temp20_volt1.150000_fix_row}.pdf}
    }
    \subcaptionbox{1.175V.}[0.31\linewidth][l]
    {
        \includegraphics[width=0.31\linewidth]{plots/figs/{hynixp65_rcd4_rp4_ret0_temp20_volt1.175000_fix_row}.pdf}
    }
    \subcaptionbox{1.2V.}[0.31\linewidth][l]
    {
        \includegraphics[width=0.31\linewidth]{plots/figs/{hynixp65_rcd4_rp4_ret0_temp20_volt1.200000_fix_row}.pdf}
    }
    \caption{Probability of observing errors due to low voltage in a DIMM from Vendor~C.}
    \label{fig:full_loc_C}
\end{figure*}
}
\section{Full Information of Every Tested DIMM}
\label{sec:dimm_info}
\tabref{modules} lists the parameters of every DRAM module that we evaluate.
\input{sections/tables/modules}
